# Supplementary material for: Open Challenges in Deep Stereo: the Booster Dataset
Source: arXiv:2206.04671 source file (2022-06-09)
Supplement: Supplementary file 1 [file supplementary.pdf]

# Supplementary Material for
# Open Challenges in Deep Stereo: the Booster Dataset

Pierluigi Zama Ramirez* Fabio Tosi* Matteo Poggi*
Samuele Salti Stefano Mattoccia Luigi Di Stefano
CVLAB, Department of Computer Science and Engineering (DISI)
University of Bologna, Italy
{pierluigi.zama, fabio.tosi5, m.poggi}@unibo.it

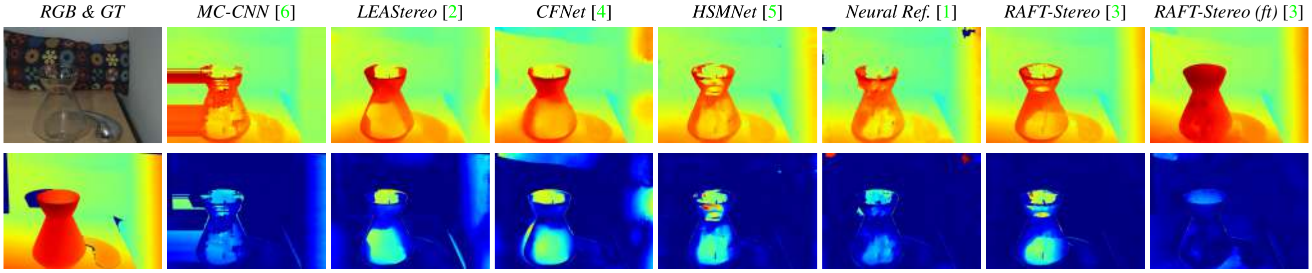


Fig. 1. **Qualitative results on Booster Unbalanced testing split.** We show the reference image (top) and ground-truth map (bottom) on leftmost column, followed by disparity (top) and error maps (bottom) for the deep models evaluated in our benchmark.

| | All pixels | | | | | |
|---|---|---|---|---|---|---|
| Category | bad-2 (%) | bad-4 (%) | bad-6 (%) | bad-8 (%) | MAE (px.) | RMSE (px.) |
| All | 55.96 | 36.81 | 27.87 | 22.33 | 9.86 | 19.36 |
| Class 0 | 53.28 | 30.31 | 19.72 | 13.04 | 5.45 | 7.62 |
| Class 1 | 63.86 | 38.31 | 25.99 | 19.18 | 6.39 | 10.41 |
| Class 2 | 76.33 | 55.93 | 40.34 | 32.52 | 17.62 | 24.12 |
| Class 3 | 84.20 | 70.31 | 60.53 | 52.64 | 27.45 | 34.62 |

Table 1. **Results on the Booster Unbalanced testing split – material segmentation.** We run RAFT-Stereo [3], using weights made available by their authors.

| | All pixels | | | | | |
|---|---|---|---|---|---|---|
| Category | bad-2 (%) | bad-4 (%) | bad-6 (%) | bad-8 (%) | MAE (px.) | RMSE (px.) |
| All | 58.67 | 32.83 | 22.96 | 17.65 | 6.31 | 11.11 |
| Class 0 | 57.04 | 27.58 | 17.36 | 12.97 | 4.72 | 7.14 |
| Class 1 | 53.17 | 30.29 | 22.32 | 17.13 | 5.16 | 7.83 |
| Class 2 | 61.90 | 40.06 | 31.54 | 26.18 | 6.71 | 10.00 |
| Class 3 | 61.40 | 42.12 | 32.50 | 26.79 | 10.56 | 14.64 |

Table 2. **Results on the Booster Unbalanced testing split after fine tuning on the training split – material segmentation.** We run RAFT-Stereo, **fine-tuned** by Booster training split.

In this document, we provide additional details concerning CVPR submission "Open Challenges in Deep Stereo: the Booster Dataset".

## 1. Unbalanced Stereo Benchmark – additional results

Because of page limit in the main paper, we report here more detailed results concerning our experiments on the Booster Unbalanced testing split, carried out in similarly to those on the Balanced testing split.

Fig. 1 we provide some qualitative results dealing with the predictions obtained by the networks evaluated in Tab. 4 of the main paper, in order to better highlight how the transparent regions represent one of the main causes of failure for a stereo network on Unbalanced split as well, and showing promising results after fine-tuning (rightmost column).

As described in the paper, material segmentation masks are warped and made available for the Unbalanced testing split as well. Thus, Tab. 1 reports error rates over the different regions, sorted in increasing degree of difficulty, achieved by RAFT-Stereo pre-trained model. Results on all valid pixels are reported on top as a reference. Consistently with the same experiment on the Balanced split, reported in Table 2 of the main paper, we can notice a consistent increase of the error metrics when going from simpler materials (class 0) to the most challenging ones (class 3). Tab.

* Joint first authorship.

| Model | All pixels bad-2 (%) | bad-4 (%) | bad-6 (%) | bad-8 (%) | MAE (px.) | RMSE (px.) |
|---|---|---|---|---|---|---|
| LEAStereo | 70.86 | 55.41 | 47.56 | 42.25 | 27.61 | 51.72 |
| LEAStereo (ft) | **62.27** | **41.96** | **32.10** | **26.28** | **20.66** | **47.29** |
| CFNet | **61.34** | 48.33 | 42.22 | 38.34 | 27.60 | 51.62 |
| CFNet (ft) | 66.94 | **46.07** | **35.50** | **29.74** | **19.65** | **43.00** |
| RAFT-Stereo | 40.27 | 27.54 | 22.83 | 20.13 | 17.08 | 36.30 |
| RAFT-Stereo (ft) | **38.68** | **23.33** | **17.66** | **14.55** | **7.56** | **17.39** |

**(a) Full res.**

| Model | All pixels bad-2 (%) | bad-4 (%) | bad-6 (%) | bad-8 (%) | MAE (px.) | RMSE (px.) |
|---|---|---|---|---|---|---|
| LEAStereo | 42.21 | 30.23 | 24.37 | 20.43 | 6.89 | 12.92 |
| LEAStereo (ft) | **26.21** | **16.13** | **12.47** | **10.46** | **5.15** | **11.80** |
| CFNet | 38.31 | 29.53 | 24.70 | 21.34 | 6.89 | 12.89 |
| CFNet (ft) | **29.64** | **19.93** | **15.59** | **12.73** | **4.78** | **10.42** |
| RAFT-Stereo | 20.13 | 15.13 | 12.85 | 11.05 | 4.27 | 9.05 |
| RAFT-Stereo (ft) | **14.46** | **9.47** | **7.32** | **5.76** | **1.87** | **4.23** |

**(b) Quarter res.**

Table 3. **Results on the Booster Balanced testing split after fine tuning on the training split** We run RAFT-Stereo, LEAStereo, and CFNET **fine-tuned** by Booster training split, processing quarter resolution images. We evaluate on full resolution ground-truth maps, or by downsampling them to quarter resolution.

| Model | All pixels bad-2 (%) | bad-4 (%) | bad-6 (%) | bad-8 (%) | MAE (px.) | RMSE (px.) |
|---|---|---|---|---|---|---|
| LEAStereo | 74.31 | 57.70 | 47.11 | 39.88 | 17.68 | 31.29 |
| LEAStereo (ft) | **67.96** | **44.90** | **32.86** | **26.38** | **14.34** | **29.27** |
| CFNet | 70.22 | 53.20 | 43.61 | 37.10 | 16.19 | 28.78 |
| CFNet (ft) | **67.31** | **46.18** | **35.18** | **28.69** | **12.99** | **27.16** |
| RAFT-Stereo | **55.96** | 36.81 | 27.87 | 22.33 | 9.86 | 19.36 |
| RAFT-Stereo (ft) | 58.67 | **32.83** | **22.96** | **17.65** | **6.31** | **11.11** |

Table 4. **Fine-tuning – unbalanced setting.**

2 reports the outcome of the same experiment, this time using RAFT-stereo weights after fine-tuning on the Booster Unbalanced training split. We can observe substantially the same trend, except for bad-2 errors. The gap on these latter across the different classes is indeed lower compared to Tab. 1. We ascribe this to the additional challenges introduced with the unbalanced setup – absent in the Balanced split.

## 2. Finetuning by the Booster training data – additional networks

We extend the experiment of Tab. 3 of the main paper, by fine-tuneing two additional networks, LEAStereo and CFNet. We report results for the unbalacend setting in Tab. 4, and for the balanced setting at full and quarter resolution in Tab. 3, validating on *All* pixels. In both tables we can notice that fine-tuning on the training split of Booster effectively improves performances for all networks in the test split, meaning that the annotation provided by our dataset help addressing the open-challenges highlighted in the paper.

## 3. Cross-verification with LiDAR sensor.

To further validate our ground-truth generation pipeline, we acquire a further scene and generate depth labels using both an Intel Realsense L515 LiDAR as well as our Space Time Stereo technique. The two are in close agreement as about 82 % of the measurements differ by less than 1 cm and the RMSE between such coherent depths is about 3.3 mm. Since the LiDAR itself is noisy, as in the main paper we measure the residuals between fitted planes and the actual depths yielded by both. Our technique turns out more accurate due to the residuals yielded by the LiDAR and our method being 0.12 and 0.05, respectively. Fig. 2 shows the two point clouds.

## 4. Dataset Samples

We add here some qualitative samples depicting the variety and complexity of our dataset.

In Fig. 3 and 4 we show 4 examples of scenes delivered with our dataset, comprising the balanced and unbalanced setup, the material segmentation mask, disparity ground-truths etc. In Fig. 5 we show point cloud visualization of the disparity maps, clearly showing the high quality of our ground-truths. Finally, in Fig. 6 we show some samples coming the 15K unlabeled images shipped with our dataset. The pictures were acquired in several different scenarios, both indoor and outdoor, with the latter acquired also in different time and weather conditions. We highlight that a lot of unlabeled frames include specular and transparent objects.

## 5. Camera Calibration Procedure

In this section, we detail the calibration procedure needed to gather images and accurate ground-truth depth labels, sketched in the leftmost block of Fig. 2 of the main paper.

**Calibration of individual cameras.** We first calibrate each camera separately using the pinhole camera model. Purposely, we acquire N images (*i.e.*, 15) containing a known pattern (*i.e.*, a chessboard) using the trinocular rig featured in Fig. 3 of the main paper.

The distortion-free projective transformation performed by a pinhole camera model is given by:

$$p = A[\mathcal{R}\mathcal{T}]P_w \tag{1}$$

where $P_w$ is a 3D point expressed according to the world reference frame (WRF), $p$ is a 2D pixel in the image plane, $A$ is the intrinsic parameters matrix and $\mathcal{R}$, $\mathcal{T}$ are the rotation and translation from the world reference frame (WRF)

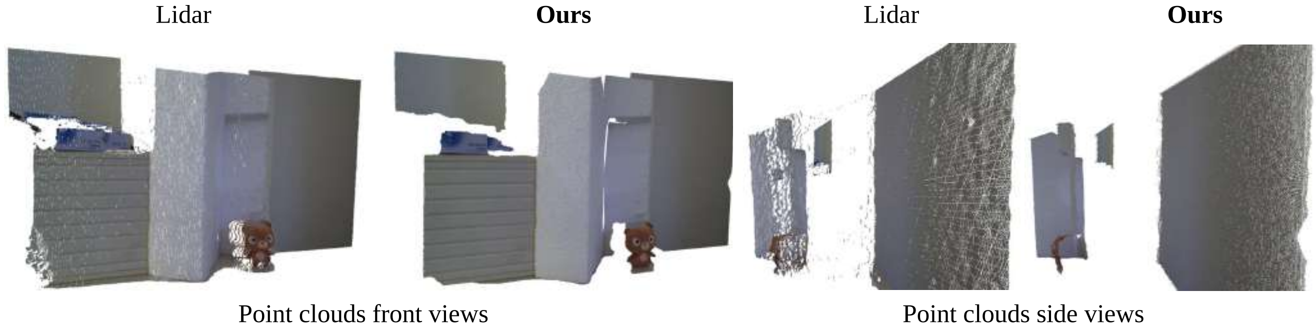


Figure 2. **Cross-verification with Intel L515 LiDAR.**

to the camera reference frame (CRF), respectively. We follow the OpenCV convention to model lens distortion by means of a vector of parameters $Dist = (k_1, k_2, k_3, p_1, p_2)$ with $k_1, k_2, k_3$ denoting the radial distortion parameters and p1,p2 the tangential distortion parameters

Given a chessboard, we can find in the images a set of key-points (*i.e.*, the inner corners of the chessboard) for which we know the exact 3D position in the WRF and, accordingly, build a set of 2D-3D correspondences. We estimate the 2D coordinates of the corners, namely $p_L, p_C, p_R$, in the L,C,R cameras, respectively, by using a standard corner detection algorithm. By calibrating independently each camera of the rig we estimate their intrinsic matrices $A_L, A_C, A_R$ and the lens distortion parameters $Dist_L$,$Dist_C$, and $Dist_R$ of the $L$,$C$, and $R$ cameras, respectively. We can then undistort the images to perform a stereo calibration of the two stereo rigs, *i.e.*, the $L - C$ and $L - R$ pairs. We can thus estimate the rotations $R_{LC}$,$R_{LR}$ and translations $T_{LC}$,$T_{LR}$, from the $L$ to $C$, and $L$ to $R$ camera reference systems, respectively.

**Balanced Stereo Calibration.** At this point, we can estimate the rectification transformations (i.e. homographies) to be applied to both images of the stereo rig to produce rectified stereo pairs. In the case of the $L - R$ *balanced* stereo system, we can address the problem as a standard rectification since the resolution is the same for both images. Thus, we rely on the OpenCV implementation to estimate the new intrinsic matrix $A_L^{LR}$ and $A_R^{LR}$, and the rotations $R_L^{LR}$ and $R_R^{LR}$ of $L$ and $R$ to map the initial image plane into the rectified image plane. We can use this information to obtain the $L_{LR}$ and $R_{LR}$ rectified stereo pair.

**Unbalanced Stereo Rectification.** To rectify images acquired by the $L - C$ unbalanced stereo system, we follow the *unbalanced rectification* scheme sketched in [1], yielding images that are rectified when brought to the same resolution by means of up-sampling or down-sampling operations solely.

We denote the camera with the smaller $HFOV$ as $j$ while the other one as $i$.

$$\begin{cases} i = L, j = C & \text{if } HFOV_C < HFOV_L \\ i = C, j = L & \text{if } HFOV_L < HFOV_C \end{cases} \tag{2}$$

By modifying the intrinsic parameters of $i$, we simulate a crop and scale of its images so as to match the $HFOV$, Aspect Ratio ($AR$) and size of $j$, and then calculate the rectification transformation based on these parameters.

Hence, we calculate the new width and height of $i$, $\hat{W}_i$ and $\hat{H}_i$, which we use to crop the image with the larger $HFOV$, thus making it matching the smaller $HFOV$ one while preserving the aspect ratio

$$\hat{W}_i = 2 \tan \frac{HFOV_j}{2} f_i \tag{3}$$

$$\hat{H}_i = \frac{H_j}{W_j} \hat{W}_i \tag{4}$$

Then, we change the intrinsic parameters of $i$ to simulate the crop and resize and thus match the resolution of $j$ as follows:

$$\hat{A}_i = \begin{bmatrix} f_x^i \cdot \frac{W_j}{\hat{W}_i} & 0 & (u_0^i - \frac{W_i - \hat{W}_i}{2}) \cdot \frac{W_j}{\hat{W}_i} \\ 0 & f_y^i \cdot \frac{H_j}{\hat{H}_i} & (v_0^i - \frac{H_i - \hat{H}_i}{2}) \cdot \frac{H_j}{\hat{H}_i} \\ 0 & 0 & 1 \end{bmatrix}$$

We estimate the rectification transformation as we would have two cameras of height $H_j$ and width $W_j$, finding the new intrinsic $A_L^{LC}$ and $A_R^{LC}$, and the rotations $R_L^{LC}$, $R_R^{LC}$, of $L$ and $C$ to map the initial image plane into the rectified one. As we have estimated the intrinsic matrices at the resolution of $j$ , we rescale $A_i^{LC}$ with a vertical and horizontal scale factors equal to $\frac{\hat{H}_i}{H_j}$ and $\frac{\hat{W}_i}{W_j}$, respectively, in order to adjust the focal length and piercing point of the camera. Finally, we can rectify the unbalanced par and thus obtain $L_{LC}$ and $C_{LC}$.

Fig. 7 shows an example of images before and after the rectification procedures described above.

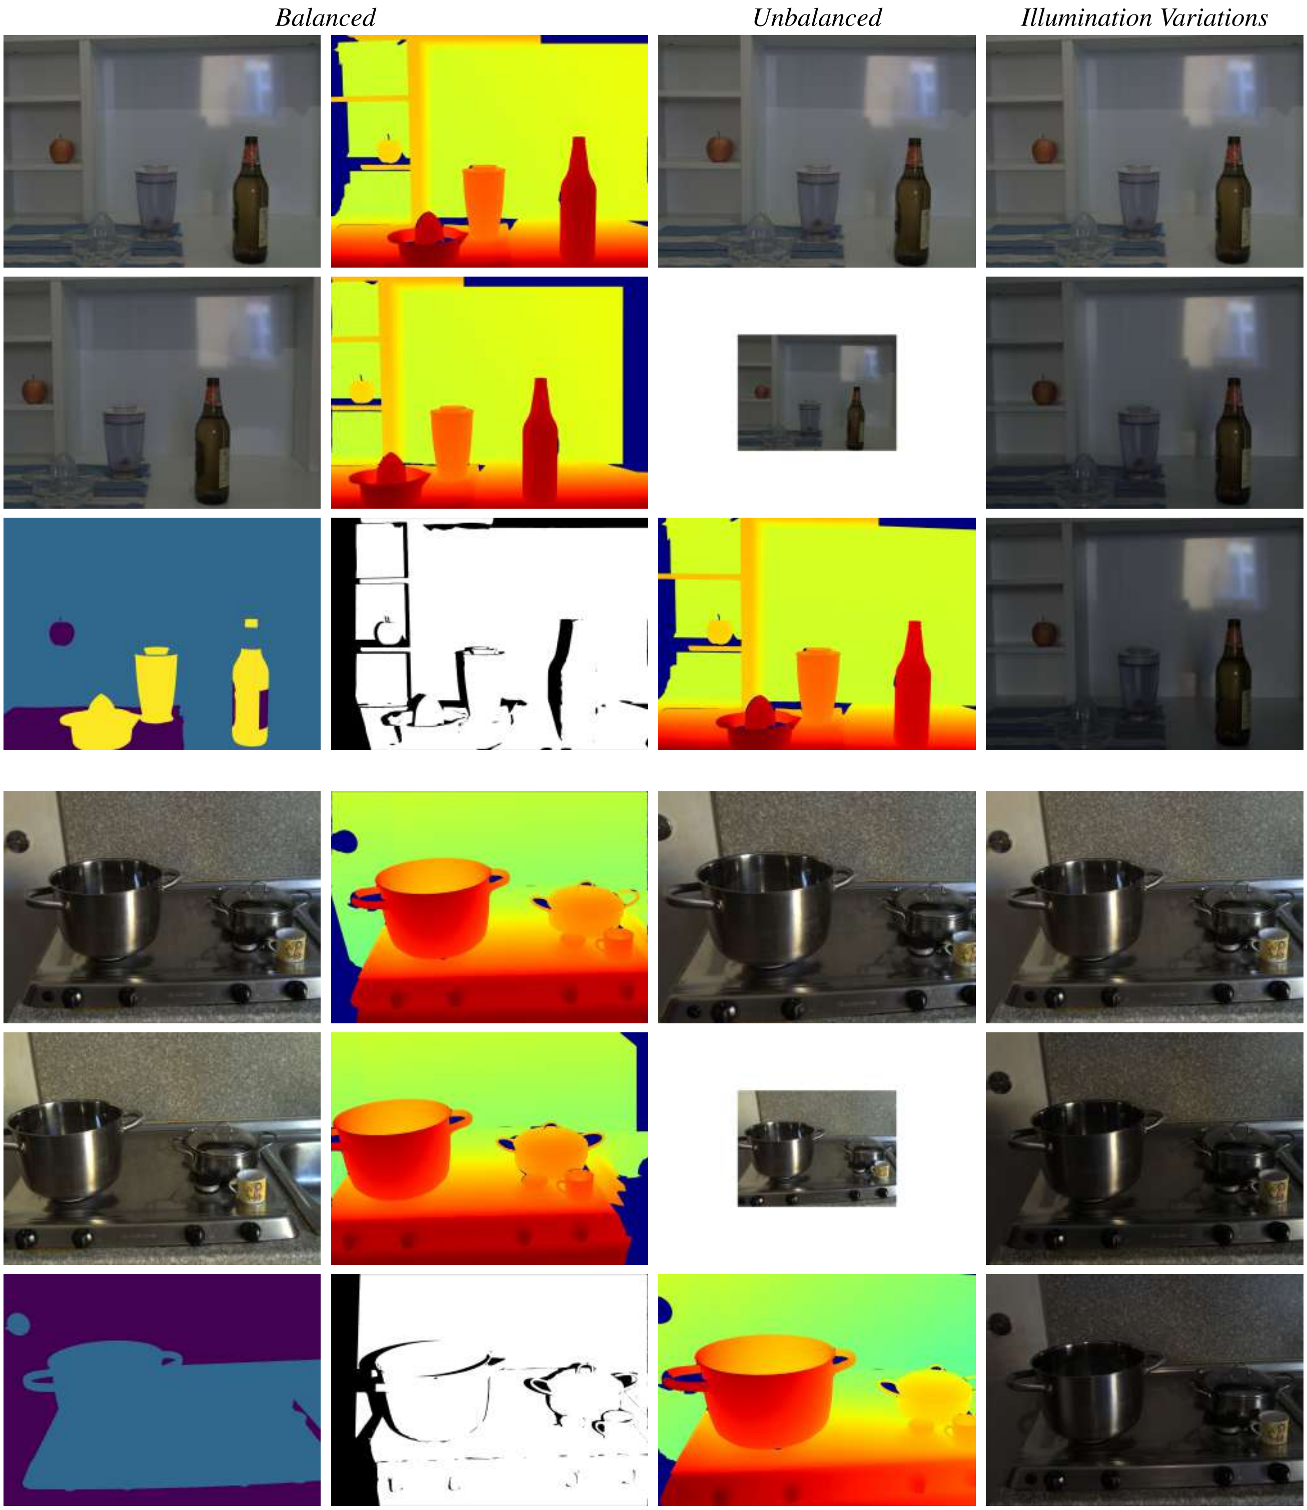


Figure 3. **Booster scene examples.** First two columns: data made available in the balanced setup (12 Mpx stereo pair, material segmentation mask, left and right disparity maps and left-right consistency mask). Third column: data dealing with the unbalanced setup (12 Mpx - 1.1 Mpx image pair, high-res disparity map associated with the 12 Mpx image ). Last columns: additional 12 Mpx images acquired under different illuminations.

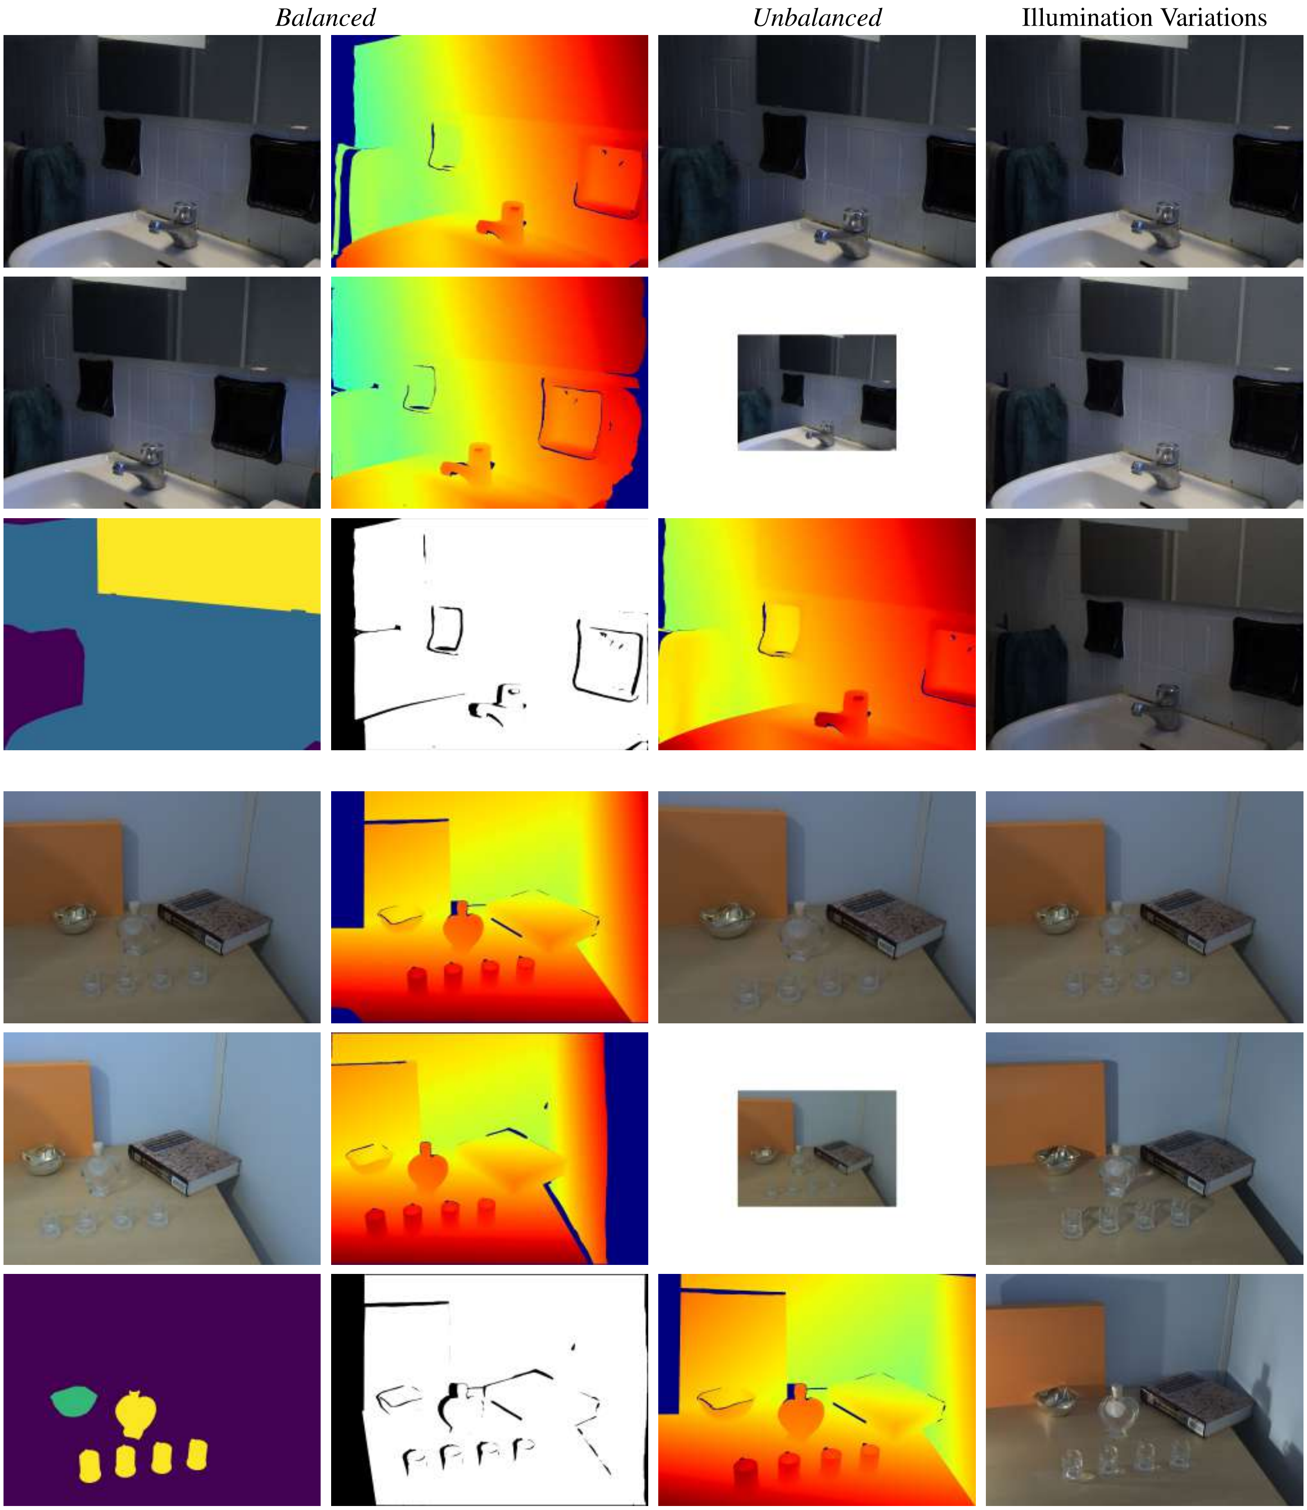


Figure 4. **Booster scene examples.** First two columns: data made available in the balanced setup (12 Mpx stereo pair, material segmentation mask, left and right disparity maps and left-right consistency mask). Third column: data dealing with the unbalanced setup (12 Mpx - 1.1 Mpx image pair, high-res disparity map associated with the 12 Mpx image ). Last columns: additional 12 Mpx images acquired under different illuminations.

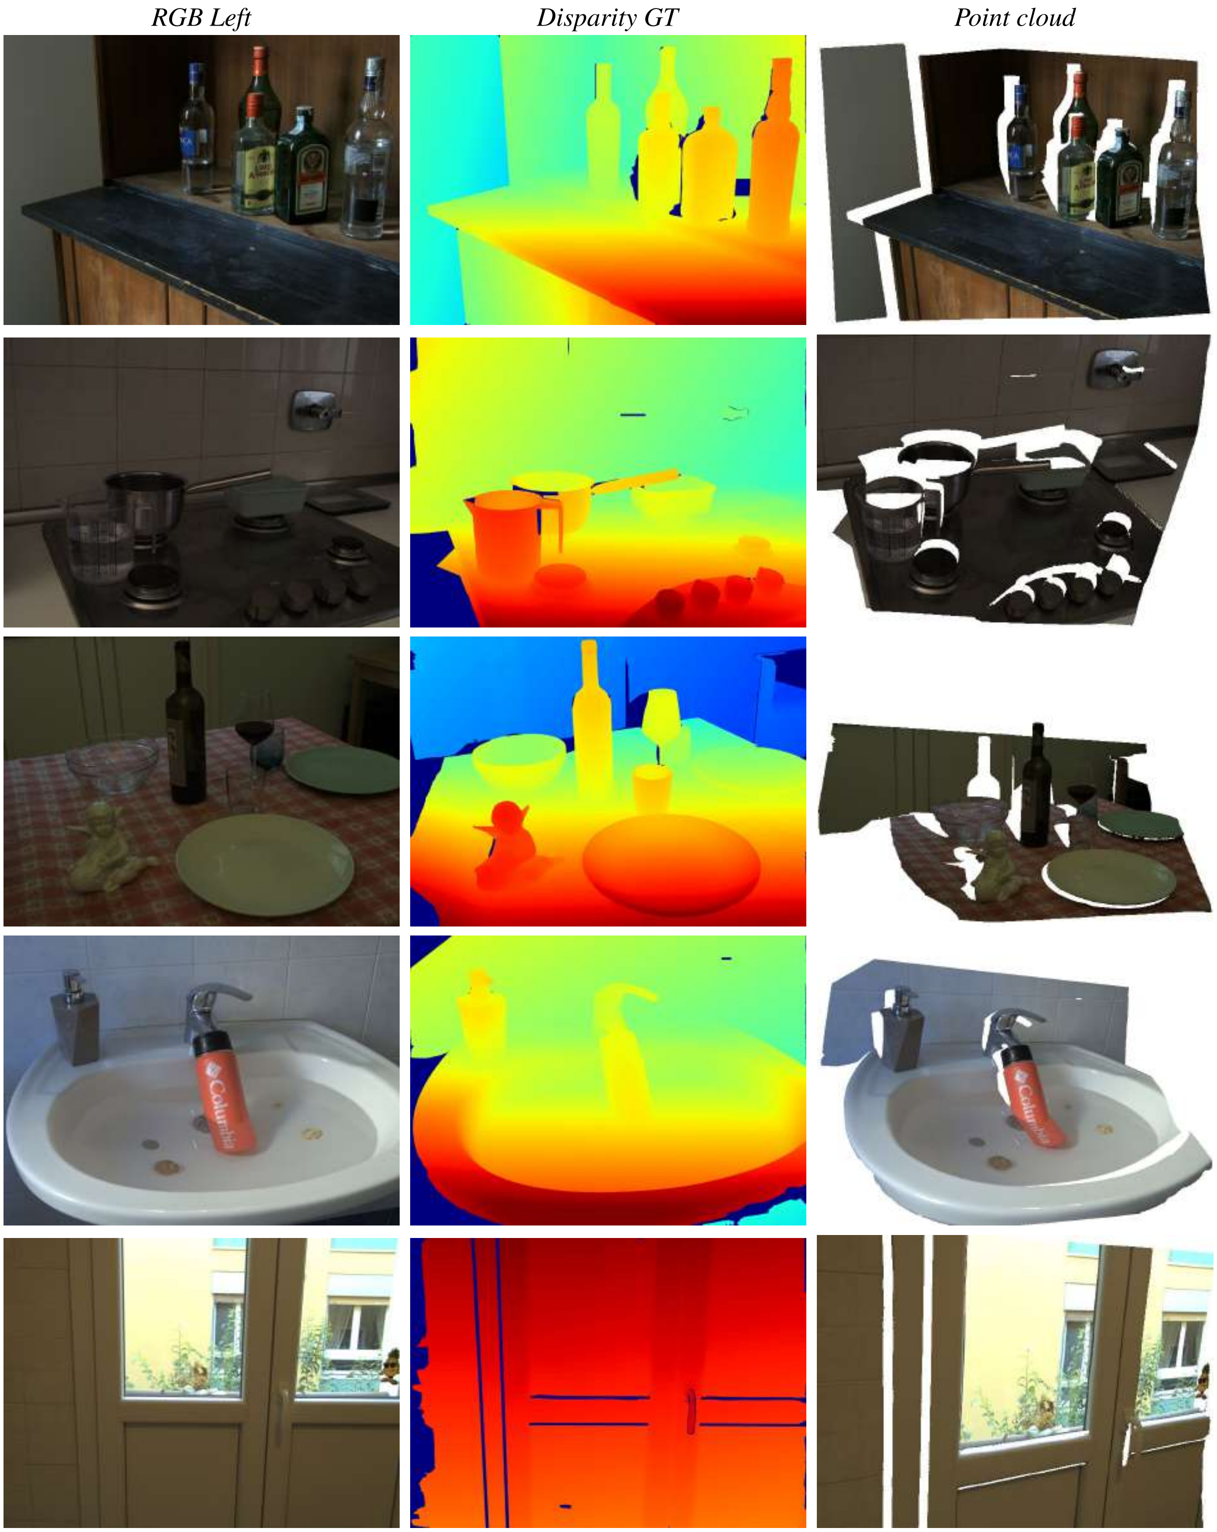


Figure 5. **Booster disparity ground-truth examples.** From left to right: RGB left image, disparity ground-truth after manual cleaning, point cloud visualization.

*Balanced Stereo Pair* *Unbalanced Stereo Pair*

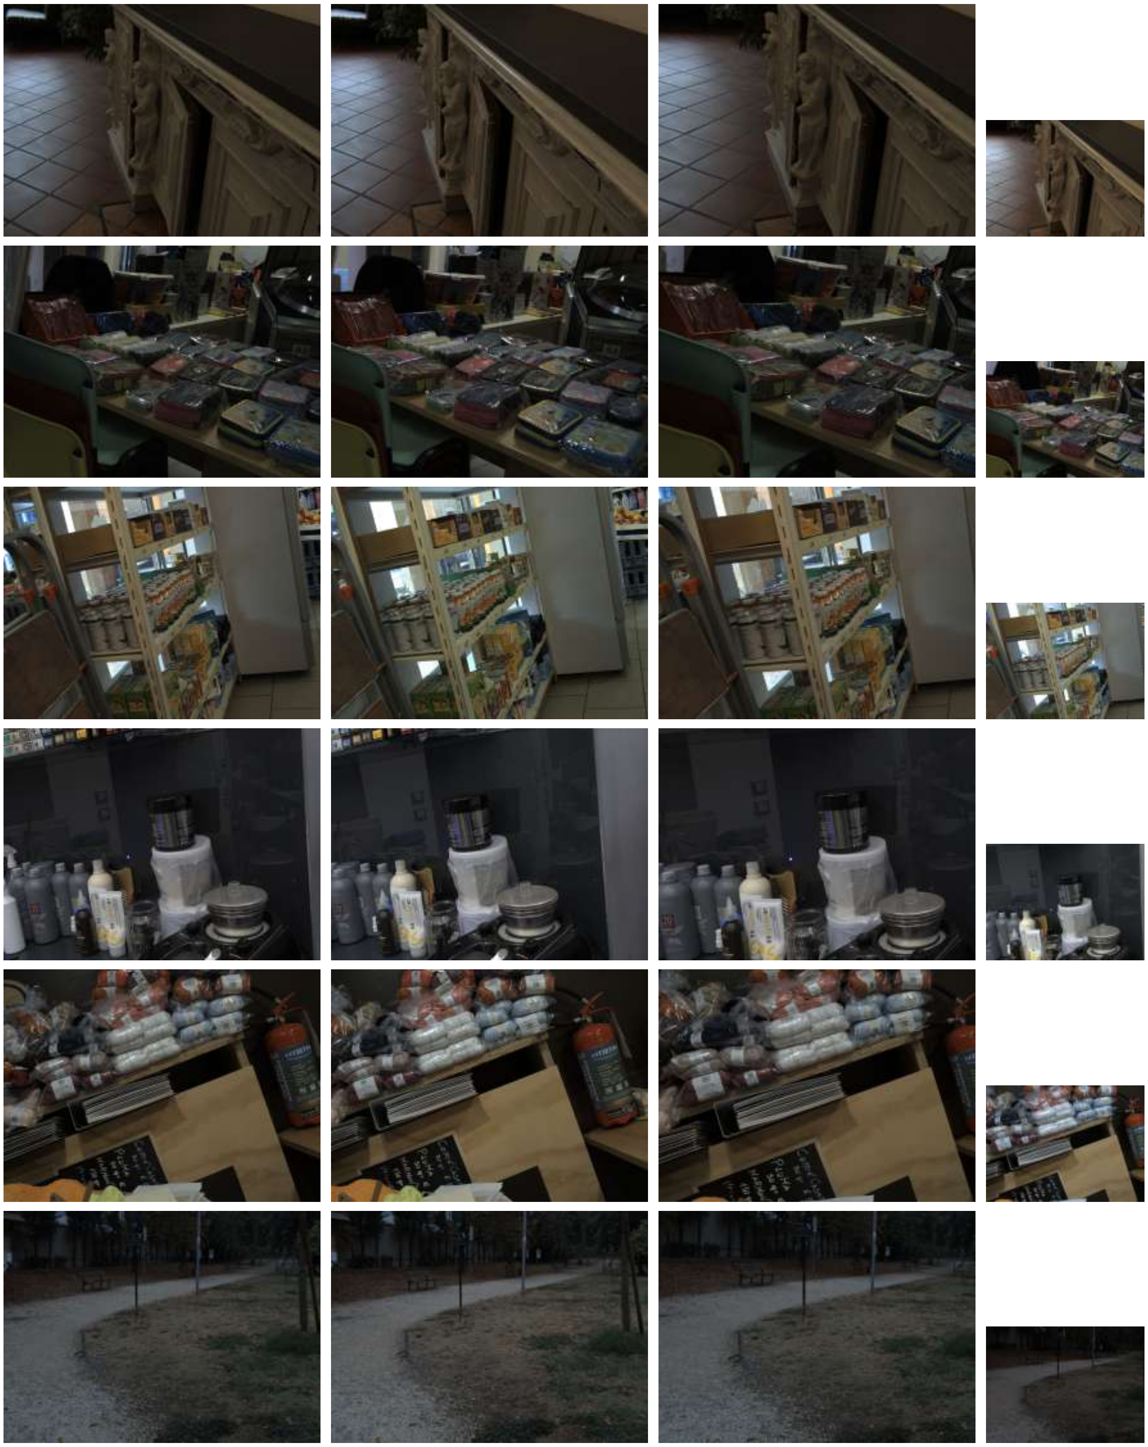

Figure 6. **Booster passive examples.** From left to right: left balanced, right balanced, left unbalanced, right unbalanced images.

## 6. Additional Details on Disparity Warping

As outlined in Sec. 3 of the main paper, in the case of the unbalanced $L-C$ stereo system, we need to warp the left ground-truth $Disp_L^{LR}$ aligned with $L-R$ to obtain the ground-truth $Disp_L^{LC}$ aligned with the left image of $L-C$.

We know that the rectification transformation is only a

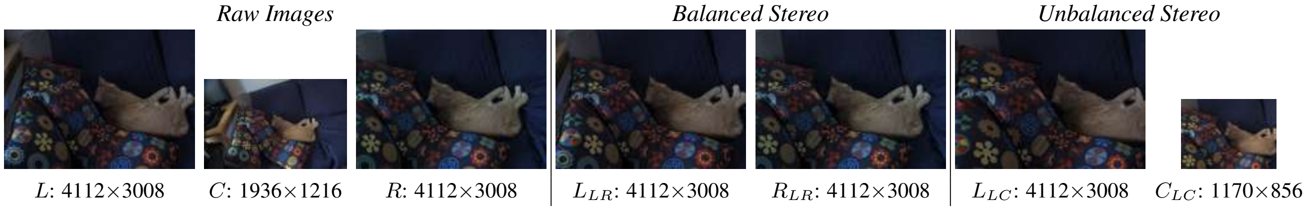


Figure 7. **Rectification example.** From left to right: $L$, $R$, and $C$ raw images acquired by our trinocular rig. $L_{LR}$,$R_{LR}$ rectified balanced stereo pair from of the $L-R$ stereo system. $L_{LC}$,$C_{LC}$ unbalanced rectified stereo pair from of the $L-C$ stereo system.

change of intrinsic parameters and a rotation, thus an homography. Therefore, we can calculate the mapping between pixels of the left image $L_{LR}$ of the $L-R$ stereo system, with coordinate $(u,v)$, and pixels of the left image $L_{LC}$ of the $L-C$ stereo system, with coordinate $(u',v')$ as:

$$\begin{pmatrix} u' \\ v' \\ 1' \end{pmatrix} = A_L^{LC} R_L^{LC} R_L^{LR^{-1}} A_L^{LR^{-1}} \begin{pmatrix} u \\ v \\ 1 \end{pmatrix} \tag{5}$$

Known this mapping we can perform a backward warping to obtain $Disp_L^{LC}$ from $Disp_L^{LR}$. However, we need to be change the disparity values according to the 3D rotation and baseline change before warping. Thus, given the disparity map $Disp_L^{LR}$ we first transform it to the corresponding depth map $D_L^{LR}$ as follows:

$$D_L^{LR} = \frac{f_{LR} b_{LR}}{Disp_L^{LR}} \tag{6}$$

Where $f_{LR}$ is the focal length of the $L_{LR}$ and $b_{LR}$ is the baseline of the stereo system $L-R$. Then, we back-project each pixel of $L_{LR}$ to 3D using $D_L^{LR}$ and we rotate it accordingly to $R$ obtaining the pixel in the $L_{LC}$ reference frame:

$$\begin{pmatrix} x' \\ y' \\ z' \end{pmatrix} = R_L^{LC} R_L^{LR^{-1}} D_L^{LR} A_L^{LR^{-1}} \begin{pmatrix} u \\ v \\ 1 \end{pmatrix} \tag{7}$$

In this way we can create a depth map $D_L^{LR\to LC}$ for which any pixel $(u,v)$ contains the depth value of the corresponding pixel aligned in the $L_{LC}$ reference frame, $z'$. At this point we perform the backward warping of the depth:

$$D_L^{LC} = \phi(D_L^{LR\to LC}) \tag{8}$$

where $\phi$ is the backward warping operation that use the mapping defined at Eq. 5 and $D_L^{LC}$ is the depth map aligned with $L_{LC}$. Finally we transform it to the ground disparity map of $L_{LC}$ as:

$$Disp_L^{LC} = \frac{f_{LC} b_{LC}}{D_L^{LC}} \tag{9}$$

where $f_{LC}$ and $b_{LC}$ are the focal length of $L_{LC}$ and the baseline of the $L-C$ stereo system.

## References


[1] Filippo Aleotti, Fabio Tosi, Pierluigi Zama Ramirez, Matteo Poggi, Samuele Salti, Luigi Di Stefano, and Stefano Mattoccia. Neural disparity refinement for arbitrary resolution stereo. In *International Conference on 3D Vision*, 2021. 3DV. 1, 3

[2] Xuelian Cheng, Yiran Zhong, Mehrtash Harandi, Yuchao Dai, Xiaojun Chang, Hongdong Li, Tom Drummond, and Zongyuan Ge. Hierarchical neural architecture search for deep stereo matching. *Advances in Neural Information Processing Systems*, 33, 2020. 1

[3] Lahav Lipson, Zachary Teed, and Jia Deng. RAFT-Stereo: Multilevel Recurrent Field Transforms for Stereo Matching. *arXiv preprint arXiv:2109.07547*, 2021. 1

[4] Zhelun Shen, Yuchao Dai, and Zhibo Rao. Cfnet: Cascade and fused cost volume for robust stereo matching. In *Proceedings of the IEEE/CVF Conference on Computer Vision and Pattern Recognition*, pages 13906–13915, 2021. 1

[5] Gengshan Yang, Joshua Manela, Michael Happold, and Deva Ramanan. Hierarchical deep stereo matching on high-resolution images. In *Proceedings of the IEEE/CVF Conference on Computer Vision and Pattern Recognition*, pages 5515–5524, 2019. 1

[6] Jure Zbontar, Yann LeCun, et al. Stereo matching by training a convolutional neural network to compare image patches. *J. Mach. Learn. Res.*, 17(1):2287–2318, 2016. 1
